# Supplementary material for: Disentangled Spatiotemporal Graph Generative Models
Source: arXiv:2203.00411 source file (2022-02-28)
Supplement: Supplementary file 1 [file appendix.tex]

\section{Supplementary Material}
\subsection{Objective Derivation}
\label{obj_proof}
\begin{proof}
First, we decompose the main objective term based on the assumption that $S_{1:T}\perp G_{1:T}|(z_{1:T},F)$ as
\begin{align}
    \mathbb{E}_{q_{\phi}(z_{1:T},F|S_{1:T}, G_{1:T})}[&\log p_{\theta}(G_{1:T}|z_{1:T},F)
    \nonumber\\&+ \log p_{\theta}(S_{1:T}|z_{1:T},F)],
    \label{infer3-1}
\end{align}
where $\perp$ indicate the conditional independent relationship. Next, considering $F=(f_{s},f_{g},f_{sg})$ and according to the assumption $S_{1:T}\perp f_g$ and $G_{1:T}\perp f_s$, we have:
\begin{align}
    \mathbb{E}_{q_{\phi}(z_{1:T},F|S_{1:T}, G_{1:T})}[&\log p_{\theta}(G_{1:T}|z_{1:T},f_{g},f_{sg})\nonumber\\
    &+ \log p_{\theta}(S_{1:T}|z_{1:T},f_{s},f_{sg})]
    \label{infer3-2}
\end{align}
Then, we extend the objective along the time dimension as:
\begin{align}
    \mathbb{E}_{q_{\phi}(z_{1:T},F|S_{1:T}, G_{1:T})&}[\log p_{\theta}(G_1,G_2,\cdots, G_T|z_{1},z_{2},\cdots,z_{T},f_g,f_{sg}) \nonumber\\
    &+\log p_{\theta}(S_1,S_2,\cdots,S_T|z_{1},z_{2},\cdots,z_{T},f_s,f_{sg})]
    \label{infer3-3}
\end{align}
We assume the snapshot graphs are independent from each other given their relevant latent representation, namely, $G_i \perp G_j|(z_i,z_j,f_g,f_{sg})$ and $S_i \perp S_j|(z_t,z_k,f_s,f_{sg})$, where $i,j\in [1,T],i\neq j $. We also have $z_{1:T} \perp (f_s, f_g, f_{sg})$, and $z_1 \perp z_2 \cdots \perp z_{T}$, the objective can be simplified as:
\begin{align}
    \mathbb{E}_{q_{\phi}(z_{1:T},F|S_{1:T}, G_{1:T})}\sum\nolimits_{t=1}^{T}&\log p_{\theta} [(G_t|z_t,f_g,f_{sg})
    \nonumber\\&+ \log p_{\theta}(S_t|z_t,f_s,f_{sg})]
    \label{infer3-5}
\end{align}

Next, by considering that $p(z_{1:T})$, $p(f_s)$, $p(f_g)$, and $p(f_{sg})$ are independent from each other given $S_{1:T}$ and $G_{1:T}$, the posterior $q_{\phi}(z_{1:T},F|S_{1:T}, G_{1:T})$ can be written as
\begin{align}
    &q_{\phi}(z_{1:T}|S_{1:T}, G_{1:T})q_{\phi}(f_{s}|S_{1:T})q_{\phi}(f_{g}|G_{1:T})q_{\phi}(f_{sg}|S_{1:T}, G_{1:T}) \nonumber\\
    &=q_{\phi}(f_g|G_{1:T})q_{\phi}(f_{s}|S_{1:T})q_{\phi}(f_{sg}|G_{1:T},S_{1:T})\prod\nolimits_{t=1}^{T}q_{\phi}(z_t|G_t,S_t).
    \label{infer3-6}
\end{align}

\end{proof}

\subsection{Proof of Theorem 1}
\label{sec:proof1}
\begin{proof}

To assist the proof, we introduce four groups of semantic factors. We assume the time-variant information is simulated via one type of semantic factor as $l_{1:T}$, time-invariant spatial-related information is simulated via two types of semantic factors as $s^+,s^-$, and time-invariant graph-related information is simulated via two parts of semantic factors as $g^+,g^-$ , which follows the convention in the disentangled representation learning domain~\cite{chen2018isolating,higgins2016beta, kim2018disentangling}. The simulation becomes $S=\textbf{Sim}(s^+,s^-,l_{1:T})$ and $G=\textbf{Sim}(g^+,g^-,l_{1:T})$. Here $s^+\perp s^-$, $g^+\perp g^-$, $s^+\perp g^+$, $s^-\nVbar g^-$, $l_{1:T}\perp g^+$, $l_{1:T} \perp g^-$, $l_{1:T} \perp s^+$, and $l_{1:T} \perp s^-$. That is, $s^+$ and $g^+$ refers to the time-invariant semantic factors of spatial and graph information, respectively. $s^-$ and $g^-$ refers to the time-invariant correlated semantic factors of spatial and graph information. $l_{1:T}$ refers to the time-variant factors of all time-variant information.

First, the objective can be rewritten based on the information bottleneck theory as:
\begin{align}
    \max_{\theta,\phi}  \quad&I(z_{1:T},f_{s},f_{sg};S_{1:T})+ I(z_{1:T},f_{g},f_{sg};G_{1:T})  \label{eq:appendix1-1}\\
    \textrm{s.t.} \quad &I(z_{1:T};S_{1:T}, G_{1:T})\leq C_t,\label{eq:appendix1-2}\\
    \quad &I(f_{s};S_{1:T})\leq I_s,\label{eq:appendix1-3}\\
    \quad &I(f_{g};G_{1:T})\leq I_g,\label{eq:appendix1-4}\\
    \quad &I(f_{sg};S_{1:T})+I(f_{sg};G_{1:T})\leq C_{sg} \label{eq:appendix1-5}
\end{align}

Due to the independence among different latent variables, the objective can be further rewritten to extend the time-invariant parts:

\begin{align}
    \max_{\theta,\phi}  \quad I(z_{1:T};S_{1:T})+I(z_{1:T};G_{1:T})+&I(f_{s},f_{sg};S_{1:T})
    \nonumber\\&+I(f_{g},f_{sg};G_{1:T}) 
    \label{eq:appendix2}
\end{align}

It is further extended as:

\begin{align}
    \max_{\theta,\phi}  \quad&I(z_{1:T};s^+)+I(z_{1:T};s^-)+2*I(z_{1:T};l_{1:T})+I(z_{1:T};g^+)\nonumber\\
    &+I(z_{1:T};g^-)+I(f_{s},f_{sg};s^+,s^-)+I(f_{s},f_{sg};l_{1:T})\nonumber\\&+I(f_{g},f_{sg};g^+,g^-)+I(f_{g},f_{sg};l_{1:T})
    \label{eq:appendix3}
\end{align}

Since $I(f_{s},f_{sg};l_{1:T}) = 0$, and $I(f_{g},f_{sg};l_{1:T}) = 0$, the time-variant information can not be expressed by the time-invariant latent variables, which are copied for all time frames. Thus, we rewrite the objective and cancel the factor as:

\begin{align}
    \max_{\theta,\phi} & \quad I(z_{1:T};s^+)+I(z_{1:T};s^-)+2*I(z_{1:T};l_{1:T})+I(z_{1:T};g^+)\nonumber\\&+I(z_{1:T};g^-)+I(f_{s},f_{sg};s^+,s^-)+I(f_{g},f_{sg};g^+,g^-) \nonumber\\
    &\quad \leq I(z_{1:T};s^+)+I(z_{1:T};s^-)+I(z_{1:T};l_{1:T})+I(z_{1:T};g^+)\nonumber\\
    &+I(z_{1:T};g^-)+I(f_{s},f_{sg};s^+,s^-)+I(f_{g},f_{sg};g^+,g^-)
    \label{eq:appendix4}
\end{align}

We rewrite constraints in Eq. \ref{eq:appendix1-1} to \ref{eq:appendix5-1}, \ref{eq:appendix5-2} and \ref{eq:appendix5-3} as:
\begin{align}
    &I(z_{1:T};s^+)+I(z_{1:T};s^-)+I(f_{s},f_{sg};s^+,s^-) \leq H(s^+, s^-) \label{eq:appendix5-1}\\
    &I(z_{1:T};g^+)+I(z_{1:T};g^-)+I(f_{g},f_{sg};g^+,g^-) \leq H(g^+, g^-)
    \label{eq:appendix5-2}\\
    &I(z_{1:T},s^+)+I(z_{1:T},s^-)+I(z_{1:T},g^+)+I(z_{1:T},g^-)\nonumber\\
    &\qquad\qquad\qquad\qquad\qquad\qquad+I(z_{1:T},l_{1:T}) \leq C_t
    \label{eq:appendix5-3}
\end{align}

We add Eq. \ref{eq:appendix5-1}, \ref{eq:appendix5-2} and \ref{eq:appendix5-3} together and have:

\begin{align}
\max_{\theta,\phi}  
    &\quad 2*I(z_{1:T},s^+)+2*I(z_{1:T},s^-)+2*I(z_{1:T},g^+)
    \nonumber\\&+2*I(z_{1:T},g^-)+I(z_{1:T},l_{1:T})+I(f_{g},f_{sg};g^+,g^-)\nonumber\\&+I(f_{s},f_{sg};s^+,s^-) \leq H(g^+,g^-)+H(s^+,s^-)+C_{t}
    \label{eq:appendix6}
\end{align}

Referring to Eq. \ref{eq:appendix4}, we have:

\begin{align}
\max_{\theta,\phi}  
    &\quad I(z_{1:T},s^+)+I(z_{1:T},s^-)+I(z_{1:T},g^+)+I(z_{1:T},g^-)\nonumber\\&+I(z_{1:T},l_{1:T})+I(f_{g},f_{sg};g^+,g^-)+I(f_{s},f_{sg};s^+,s^-) \nonumber\\&\leq H(g^+,g^-)+H(s^+,s^-)+C_{t}
    \label{eq:appendix6+1}
\end{align}

Since $H(g^+,g^-)+H(s^+,s^-)+C_t > 0$, $I(z_{1:T},g^+) \geq 0$, $I(z_{1:T},g^+) \geq 0$, $I(z_{1:T},s^+) \geq 0$, $I(z_{1:T},s^-) \geq 0$, and we ignore the time-invariant part, $I(f_{g},f_{sg};g^+,g^-) +I(f_{s},f_{sg};s^+,s^-)$ for now, only when $I(z_{1:T},g^+)+I(z_{1:T},g^+)+I(z_{1:T},s^+)+I(z_{1:T},s^-) = 0$, the left-hand side of the Inequality Eq. \ref{eq:appendix6+1} reaches the maximum for time-variant variables. Thus, the maximum is achieved only when the time-variant variables $z_{1:T}$ have no correlation with any of the time-invariant variables. Next, we deal with the time-invariant part, the objective function becomes:

\begin{align}
    \max_{\theta,\phi}  
    \quad I(f_{g},f_{sg};g^+,g^-)+I(f_{s},f_{sg};s^+,s^-)+I(z_{1:T},l_{1:T})
    \label{eq:appendix7}
\end{align}

Now, we extend the time-invariant spatial, graph and joint variables as:

\begin{align}
    \max_{\theta,\phi}  
    &\quad I(f_{g},f_{sg};g^+,g^-)=I(f_{g},g^+)+I(f_{g},g^-)\nonumber\\&+I(f_{sg},g^+)+I(f_{sg},g^-) \nonumber\\
    &I(f_{s},f_{sg};s^+,s^-)=I(f_{s},s^+)+I(f_{s},s^-)
    \nonumber\\&+I(f_{sg},s^+)+I(f_{sg},s^-) 
    \label{eq:appendix8}
\end{align}

Since $f_{s} \perp z_{1:T}$ and $s^- \nVbar g^-$, we have $I(f_{s},s^-)=0$ and $I(f_{g},g^-)=0$, the object can be rewritten as:
\begin{align}
    \max_{\theta,\phi}  
    &\quad I(f_{g},g^+)+I(f_{sg},g^+)+I(f_{sg},g^-)+I(f_{s},s^+)
    \nonumber\\&+I(f_{sg},s^+)+I(f_{sg},s^-)+I(z_{1:T},l_{1:T})
    \label{eq:appendix9}
\end{align}

Since $f_{s} \perp f_{sg}$ and $f_{g} \perp f_{sg}$, there is no mutual information between information in $s^+$ captured by $f_{s}$ and information in $s^+$ captured by $f_{sg}$, the Eq. 9, 10 become:

\begin{align}
    I(f_{s};s^+)+I(f_{sg},s^+) \leq I(s^+;s^+)=H(s^+) \nonumber\\
    I(f_{g};g^+)+I(f_{sg},g^+) \leq I(g^+;g^+)=H(g^+) \label{eq:appendix10}
\end{align}

The constraint in Eq. \ref{eq:appendix1-5} is equivalent to Eq. \ref{eq:appendix11}:
\begin{align}
    I(f_{sg};s^+)+I(f_{sg},s^-)+I(f_{sg};g^+)+I(f_{sg},g^-) \leq C_{sg}
    \label{eq:appendix11}
\end{align}

By adding Eq. \ref{eq:appendix10} and Eq. \ref{eq:appendix11}, we have:

\begin{align}
    &I(f_{s};s^+)+2*I(f_{sg},s^+)+I(f_{sg};s^-)+I(f_{g},g^+)\nonumber\\&+2*I(f_{sg},g^+)+I(f_{sg},g^-)\leq H(s^+)+H(g^+)+C_{sg}
    \label{eq:appendix12}
\end{align}

To rewrite it by canceling the factors, we get:
\begin{align}
    &I(f_{s};s^+)+I(f_{sg};s^+)+I(f_{g},g^+)+I(f_{g},g^-)+I(f_{sg},s^+)\nonumber\\
    &+I(f_{sg},g^+)\leq H(s^+)+H(g^+)+C_{sg}
    \label{eq:appendix13}
\end{align}

Since $I(z_{sg};s^+) \geq 0$ and $I(z_{sg_g};g^+) \geq 0$, and $H(s^+)$, $H(g^+)$ are constants, only when $I(z_{sg};s^+)=0$ and $I(z_{sg};g^+)=0$, the Inequality Eq. \ref{eq:appendix13} reaches the maximum. Therefore, only when $z_{sg}$ only captures information from spatial-graph joint semantic factors $s^+$ and $g^+$, the optimum of the objective is reached.

Overall, only when the time-variant variables $z_{1:T}$ have no correlation with any of the time-invariant variables and $z_{sg}$ only captures information from time-invariant spatial-graph joint semantic factors $s^+$ and $g^+$, the optimum of the objective is reached.

\end{proof}

\subsection{Proof of Theorem 2}
\label{sec:proof2}

\begin{proof}
First, at the initial stage, $\mathcal{R}_3=0$ and  $\mathcal{R}_2=0$, we then gradually increase $I_t$ and $I_{sg}$, and at each step while well-trained,  $\prod\nolimits_{t=1}^{T} D_{KL}(q_{\phi}(z_{t}|G_t,S_t)||p(z_t))$ and $ D_{KL}(q_{\phi}(f_{sg}|G_{1:T},S_{1:T})||p(f_{sg}))$ will keep increasing to catch $I_t$ and $I_{sg}$.  

Next, when $\mathcal{R}_3<0$ and  $\mathcal{R}_2<0$, namely the information that captured by $I_t$ and $I_{sg}$ do not increase anymore, we can conclude that $I_t=C_t$ and $I_{sg}=C_{sg}$ (proved as follows). Thus, the whole optimization process can be stopped. During the whole process, the two constraint $I_{t} \leq C_{t}$ and $I_{sg} \leq C_{sg}$ are always satisfied, namely, the $z_t$ always captures and only captures time-variant information and $f_{sg}$ always captures and only captures time-invariant spatial-graph correlated information. 

Here we prove that when the information that captured by $I_t$ and $I_{sg}$ do not increase anymore, it indicates that $I_t=C_t$ and $I_{sg}=C_{sg}$ and we have achieved the optimal objective. 
To assist the proof, we introduce four groups of semantic factors. We assume the time-variant information is simulated via one type of semantic factor as $l_{1:T}$, time-invariant spatial-related information is simulated via two types of semantic factors as $s^+,s^-$, and time-invariant graph-related information is simulated via two parts of semantic factors as $g^+,g^-$ , which follows the convention in the disentangled representation learning domain~\cite{chen2018isolating,higgins2016beta, kim2018disentangling}. The simulation becomes $S=\textbf{Sim}(s^+,s^-,l_{1:T})$ and $G=\textbf{Sim}(g^+,g^-,l_{1:T})$. Here $s^+\perp s^-$, $g^+\perp g^-$, $s^+\perp g^+$, $s^-\nVbar g^-$, $l_{1:T}\perp g^+$, $l_{1:T} \perp g^-$, $l_{1:T} \perp s^+$, and $l_{1:T} \perp s^-$. That is, $s^+$ and $g^+$ refers to the time-invariant semantic factors of spatial and graph information, respectively. $s^-$ and $g^-$ refers to the correlated semantic factors of spatial and graph information.

(1) Given $z_{1:T}$ captures all the time-variant semantic factors, namely $\prod\nolimits_{t=1}^{T} D_{KL}(q_{\phi}(z_{t}|G_t,S_t)||p(z_t))=c_{t}$, the information captured by $z_t$ will not increase anymore, we have $I(z_{1:T},l_{1:T})=I(l_{1:T},l_{1:T})$; Given $f_s$ captures all the time-invariant spatial-independent semantic factors $s^+$, namely $D_{KL}(q_{\phi}(f_{sg}|G_{1:T},S_{1:T})||p(f_{sg}))$, the information captured by $f_{sg}$ will not increase anymore, and we have $I(f_s,s^+)=I(s^+,s^+)$; Given $f_g$ captures all the time-invariant graph-independent semantic factors $g^+$, we have $I(f_g,g^+)=I(g^+,g^+)$; Given $f_{sg}$ captures all the time-invariant spatial-graph correlated semantic factors $s^-$, $g^-$, we have $I(f_{sg},s^+)=0$, $I(f_{sg},g^+)=0$, and $I(f_{sg},s^-)=I(s^-,s^-)$, $I(f_{sg},g^-)=I(g^-,g^-)$. Thus, the value of already achieved loss is equal to $I(s^+,s^+)+I(s^-,s^-)+I(g^+,g^+)+I(g^-,g^-)+I(l_{1:T},l_{1:T})$. (2) Next, we rewrite the original objective function as follows:
\begin{align}
    \max_{\theta,\phi}  \quad&I(z_{1:T};s^+)+I(z_{1:T};s^-)+2*I(z_{1:T};l_{1:T})
    \nonumber\\&+I(z_{1:T};g^+)+I(z_{1:T};g^-)+I(f_{s},s^+)+I(f_{sg},s^+)\nonumber\\&+I(f_{sg},s^-)+I(f_{g},g^+)+I(f_{sg},g^+)+I(f_{sg},g^-)\nonumber\\
    &+I(f_{s},l_{1:T})+I(f_{sg},l_{1:T})+I(f_{g},l_{1:T})
    \label{eq:appendix14}
\end{align}
Since $f_s \perp f_{sg}$, $f_g \perp f_{sg}$ and $z_{1:T} \perp f_s$, $z_{1:T} \perp f_g$, $z_{1:T} \perp f_{sg}$, we have:
\begin{align}
    I(f_s, s^+)+I(f_{sg}, s^+)+I(z_{1:T},s^+)\leq I(s^+,s^+) \\
    I(f_g, g^+)+I(f_{sg}, g^+)+I(z_{1:T},g^+)\leq I(g^+,g^+) \\
    I(f_{sg}, s^-)+I(z_{1:T},s^-)\leq I(s^-,s^-) \\
    I(f_{sg}, g^-)+I(z_{1:T},g^-)\leq I(g^-,g^-) \\
     I(z_{1:T}, l_{1:T})\leq I(l_{1:T},l_{1:T})
\end{align}
Thus, the optimal loss is $I(s^+,s^+)+I(s^-,s^-)+I(g^+,g^+)+I(g^-,g^-)+I(l_{1:T},l_{1:T})$. In this situation, the optimal loss is already achieved. If we continue increase $I_t$ and $I_{sg}$, the information captured by $z_t$ and $f_{sg}$ will not increase anymore, thus we got $\mathcal{R}_2<0$ and $\mathcal{R}_3<0$. which is a signal for stopping the optimization process.

\end{proof}

\subsection{Time-dependent Objective Function}
\label{sec:time_dep}

As demonstrated in section \ref{sec:obj}, the objective leads to the maximization problem below:
\begin{align}
    &\max_{\theta,\phi} \quad \mathbb{E}_{S_{1:T}, G_{1:T}\sim D}[\mathbb{E}_{q_{\phi}(z_{1:T}, F|S_{1:T}, G_{1:T})}
    \nonumber\\&\qquad\qquad\qquad\qquad log p_{\theta}(S_{1:T}, G_{1:T}|z_{1:T},f_{s},f_{g},f_{sg})]   \nonumber\\
    &\textrm{s.t.}\quad D_{KL}(q_{\phi}(z_{1:T},F|S_{1:T}, G_{1:T})||p(z_{1:T},f_{s},f_{g},f_{sg})<\epsilon
\end{align}
where $D$ refers to the observed dataset of the spatial network dynamics.\normalsize
This is equal to maximize the evidence lower-bound (ELBO), as follows:
\begin{align}
    &\max_{\theta,\phi} \quad \mathbb{E}_{S_{1:T}, G_{1:T}\sim D}[\mathbb{E}_{q_{\phi}(z_{1:T}, F|S_{1:T}, G_{1:T})}\nonumber\\
    &\qquad\qquad\qquad\qquad log p_{\theta}(S_{1:T}, G_{1:T}|z_{1:T},f_{s},f_{g},f_{sg})]   \nonumber\\
    &- \lambda D_{KL}(q_{\phi}(z_{1:T},f_{s},f_{g},f_{sg}|S_{1:T}, G_{1:T})||p(z_{1:T},f_{s},f_{g},f_{sg})
\end{align}

First, we decompose the main objective term based on the assumption that $S_{1:T}\perp G_{1:T}|(z_{1:T},f_s,f_g,f_{sg})$:
\begin{align}
        % &\mathbb{E}_{q_{\phi}(z_{1:T},F|S_{1:T}, G_{1:T})}[\log p_{\theta}(S_{1:T}, G_{1:T}|z_{1:T},f_{s},f_{g},f_{sg})]\nonumber\\
        \mathbb{E}_{q_{\phi}(z_{1:T},F|S_{1:T}, G_{1:T})}&[\log p_{\theta}(G_{1:T}|z_{1:T},f_{s},f_{g},f_{sg})
        \nonumber\\&+ \log p_{\theta}(S_{1:T}|z_{1:T},f_{s},f_{g},f_{sg})]
\end{align}
According to the assumption $S_{1:T}\perp f_g$ and $G_{1:T}\perp f_s$, we have:
\begin{align}
    \mathbb{E}_{q_{\phi}(z_{1:T},F|S_{1:T}, G_{1:T})}&[\log p_{\theta}(G_{1:T}|z_{1:T},f_{g},f_{sg})\nonumber\\
    &+ \log p_{\theta}(S_{1:T}|z_{1:T},f_{s},f_{sg})]
\end{align}
Then, we extend the objective through the time dimension as:
\begin{align}
    \mathbb{E}_{q_{\phi}(z_{1:T},F|S_{1:T}, G_{1:T})&}[\log p_{\theta}(G_1,G_2,\cdots, G_T|z_{1},z_{2},\cdots,z_{T},f_g,f_{sg}) \nonumber\\
    &+\log p_{\theta}(S_1,S_2,\cdots,S_T|z_{1},z_{2},\cdots,z_{T},f_s,f_{sg})]
\end{align}
Since the sequence is dependent through time, $z_1 \nVbar z_2 \cdots \nVbar z_{T}$, we simplify the objective as:
\begin{align}
    &\mathbb{E}_{q_{\phi}(z_{1:T},F)|S_{1:T}, G_{1:T})}[\log p_{\theta}(G_{1}|z_{1},f_{g},f_{sg})p_{\theta}(z_{2}|z_{1})\nonumber\\
    &\qquad\qquad\qquad\qquad\qquad\cdots p_{\theta}(z_{T}|z_{T-1})p_{\theta}(G_{T}|z_{T},f_{g},f_{sg})\nonumber\\
    &+\log p_{\theta}(S_{1}|z_{1},f_{s},f_{sg})p_{\theta}(z_{2}|z_{1})\cdots p_{\theta}(z_{T}|z_{T-1})p_{\theta}(S_{T}|z_{T},f_{s},f_{sg})]
\end{align}

We re-organize the objective by putting the product together as:

\begin{align}
    &\mathbb{E}_{q_{\phi}(z_{1:T},F)|S_{1:T}, G_{1:T})}[\log \prod_{t=1}^{T} p_{\theta}(G_t|z_t,f_{g},f_{sg})\prod_{t=2}^{T}p_{\theta}(z_t|z_{t-1})
    \nonumber\\
    &\qquad\qquad+\log \prod_{t=1}^{T} p_{\theta}(S_t|z_t,f_{s},f_{sg})\prod_{t=2}^{T}p_{\theta}(z_t|z_{t-1})]
\end{align}

Finally, the objective is written as the following by taking the product out of log function as summation: 
\begin{align}
    &\mathbb{E}_{q_{\phi}(z_{1:T},F)|S_{1:T}, G_{1:T})}[\sum_{t=1}^{T} \log  p_{\theta}(G_t|z_t,f_{g},f_{sg})\nonumber\\
    &+ \sum_{t=2}^{T} \log p_{\theta}(z_t|z_{t-1})+\sum_{t=1}^{T}\log  p_{\theta}(S_t|z_t,f_{s},f_{sg})\nonumber\\
    &+\log \sum_{t=2}^{T}p_{\theta}(z_t|z_{t-1})]
\end{align}

Next, we extend the encoder part $q_{\phi}(z_{1:T},F|S_{1:T}, G_{1:T})$ $F$ to $f_s$, $f_g$, and $f_{sg}$, and decompose it based on the assumption that $p(z_{1:T})$ and $p(f_s)$, $p(f_g)$, and $p(f_{sg})$ are independent given $S_{1:T}$ and $G_{1:T}$ as:
\begin{align}
    &q_{\phi}(z_{1:T},f_s,f_g,f_{sg}|S_{1:T}, G_{1:T}) =q_{\phi}(z_{1:T}|S_{1:T}, G_{1:T})q_{\phi}(f_{s}|S_{1:T})\nonumber\\
    &p_{\phi}(f_{g}|G_{1:T})q_{\phi}(f_{sg}|S_{1:T}, G_{1:T}) =q_{\phi}(z_1|G_{1},S_{1})q_{\phi}(z_2|z_{1},G_{2},S_{2})
    \nonumber\\&q_{\phi}(z_3|z_{2},G_{3},S_{3})
    \cdots q_{\phi}(z_{T}|z_{T-1},S_{T},G_{T})q_{\phi}(f_{s}|S_{1:T})q_{\phi}(f_{g}|G_{1:T})\nonumber\\&q_{\phi}(f_{sg}|S_{1:T}, G_{1:T})=\prod_{t=2}^{T} q_{\phi}(z_{t}|z_{t-1},S_{t}, G_{t})q_{\phi}(z_{1}|S_1,G_1)\nonumber\\&\prod_{t=1}^{T}q_{\phi}(f_{s}|S_t)p_{\phi}(f_{g}|G_t)q_{\phi}(f_{sg}|S_{t}, G_{t})
\end{align}
Then the objective is written as:
\begin{align}\nonumber
   \label{eq:initial_objective}
    &\max_{\theta,\phi} \quad\mathbb{E}_{S_{1:T}, G_{1:T}\sim D}\mathbb{E}_{q_{\phi}(z_{1:T},F|S_{1:T},G_{1:T})}
    \nonumber\\&[\sum_{t=1}^{T} \log  p_{\theta}(G_t|z_{t},f_g,f_{sg})+\sum_{t=2}^{T} \log p_{\theta}(z_{t}|z_{t-1})\nonumber\\&
    +\sum_{t=1}^{T}\log  p_{\theta}(S_t|z_{t},f_s,f_{sg})+\log \sum_{t=2}^{T}p_{\theta}(z_{t}|z_{t-1})] \nonumber\\
    &\textrm{s.t.} \; D_{KL}(\prod_{t=2}^{T}q_{\phi}(z_{t}|z_{t-1},S_{t}, G_{t})q_{\phi}(z_1|S_1,G_1)||p(z_{1:T}))<I_t.\nonumber\\
    & \quad D_{KL}(q_{\phi}(f_{g}|G_{1:T})||p(f_{g}))<I_g.\nonumber\\
    & \quad D_{KL}(q_{\phi}(f_{s}|S_{1:T})||p(f_{s}))<I_s \nonumber\\
    & \quad D_{KL}(q_{\phi}(f_{sg}|S_{1:T}, G_{1:T})||p(f_{sg}))<I_{sg} 
\end{align}

Next, we focus on the first constrain on time. Since $z_t$ are dependent on each other, we assume a conditional prior distribution of $z_t$ instead of Normal distribution. That is, $p(z_t|z_{t-1})\sim \mathcal{N}(\mu(z_{t-1}); \sigma(z_{t-1}))$. Here $\mu(\cdot)$ and $\sigma(\cdot)$ can be implemented by any functions like neural networks. And $p(z_1)\sim \mathcal{N}(0; 1)$. Thus, we further decompose the first constrain as:

where $D_{KL}(\prod_{t=2}^{T} q_{\phi}(z_{t}|z_{t-1},S_{T}, G_{T})q_{\phi}(z_1|S_1,G_1)||p(z_{1:T}))$ is derived by:
\begin{align}
    &D_{KL}(\prod_{t=2}^{T} q_{\phi}(z_{t}|z_{t-1},S_{T}, G_{T})q_{\phi}(z_1|S_1,G_1)||p(z_{1:T}))\nonumber\\
    &=D_{KL}(q_{\phi}(z_1|S_1,G_1),q_{\phi}(z_{2}|z_{1},S_{2}, G_{2}),\cdots,
    \nonumber\\&q_{\phi}(z_{t}|z_{t-1},S_{t}, G_{t})||p(z_1),p(z_1|z_2),\cdots,p(z_{t-1}|z_t))\nonumber\\
    &=\sum_{z} q_{\phi}(z_1|S_1,G_1)q_{\phi}(z_{2}|z_{1},S_{2}, G_{2})\cdots q_{\phi}(z_{t}|z_{t-1},S_{t}, G_{t})\nonumber\\&\log \frac{q_{\phi}(z_1|S_1,G_1)q_{\phi}(z_{2}|z_{1},S_{2}, G_{2})\cdots q_{\phi}(z_{t}|z_{t-1},S_{t}, G_{t})}{p(z_1)p(z_1|z_2)\cdots p(z_{t-1}|z_t)}\nonumber\\
    &=E[\log \frac{q_{\phi}(z_1|S_1,G_1)q_{\phi}(z_{2}|z_{1},S_{2}, G_{2})\cdots q_{\phi}(z_{t}|z_{t-1},S_{t}, G_{t})}{p(z_1)p(z_1|z_2)\cdots p(z_{t-1}|z_t)}]\nonumber\\
    &=E[\log {q_{\phi}(z_1|S_1,G_1)q_{\phi}(z_{2}|z_{1},S_{2}, G_{2})\cdots q_{\phi}(z_{t}|z_{t-1},S_{t}, G_{t})} \nonumber\\&\qquad\qquad\qquad- \log{p(z_1)p(z_1|z_2)\cdots p(z_{t-1}|z_t)}]\nonumber\\&=E[\log {q_{\phi}(z_1|S_1,G_1)q_{\phi}(z_2|z_1,S_2,G_2)\cdots q_{\phi}(z_T|z_{T-1},S_T,G_T)} \nonumber\\&\qquad\qquad\qquad- \log{p(z_{1})p(z_2|z_1)\cdots p(z_T|z_{T-1}))}]\nonumber\\
    &=E[\log \prod\nolimits_{t=2}^{T}{q_{\phi}(z_t|z_{t-1},S_t,G_t)}q_{\phi}(z_1|,S_1,G_1) \nonumber\\&\qquad\qquad\qquad- \log{\prod\nolimits_{t=2}^{T} p(z_{t}|z_{t-1})p(z_1)}]\nonumber\\
    &=E[\sum\nolimits_{t=2}^{T} \log {q_{\phi}(z_t|z_{t-1},S_t,G_t)}+ \log{q_{\phi}(z_1|S_1,G_1)} \nonumber\\&\qquad\qquad\qquad - \sum\nolimits_{t=2}^{T} \log{ p(z_{t}|z_{t-1}) }+\log{p(z_1)}]\nonumber\\
    &=\sum\nolimits_{t=2}^{T} E[\log \frac{q_{\phi}(z_t|z_{t-1},S_t,G_t)}{p(z_{t}|z_{t-1})} + \log \frac{q_{\phi}(z_1|,S_1,G_1)}{p(z_{1})}]\nonumber\\
    &=\sum\nolimits_{t=2}^{T} D_{KL}(q_{\phi}(z_t|z_{t-1},S_t,G_t)||p(z_t|z_{t-1}))\nonumber\\&\qquad\qquad\qquad + D_{KL}(q_{\phi}(z_1|S_t,G_t)||p(z_1))
    \label{infer7}
\end{align}

% \textbf{As we are using RNN, so the condition actually is not like what we expect before (encoding from Zt to Z1, decoding from Z1 to Zt), now we are (encoding Z1 to Zt, decoding Z1 to Zt)}
% The final objective function is as follows:
% \begin{align}\nonumber
%   \label{eq:initial_objective}
%     \max_{\theta,\phi} \quad&\mathbb{E}_{S_{1:T}, G_{1:T}\sim D}\mathbb{E}_{\prod_{t=1}^{T-1} (q_{\phi}(z_{1:T}|z_{t+1},S_{1:T}, G_{1:T}))q_{\phi}(z_{1:T}|t,s)\prod_{t=1}^{T}q_{\phi}(f_{s}|s)p_{\phi}(f_{g}|g)q_{\phi}(f_{sg}|S_{1:T}, G_{1:T})}[\sum_{t=1}^{T} \log  p_{\theta}(t|z_{1:T},f_g,f_{sg})+ \sum_{t=2}^{T} \log p_{\theta}(z_{1:T}|z_{t-1})+\sum_{t=1}^{T}\log  p_{\theta}(s|z_{1:T},f_s,f_{sg})+\log \sum_{t=2}^{T}p_{\theta}(z_{1:T}|z_{t-1})] \\\nonumber
%     &-\lambda D_{KL}(\prod_{t=1}^{T-1} (q_{\phi}(z_{1:T}|z_{t+1},S_{1:T}, G_{1:T}))q_{\phi}(z_{1:T}|t,s)||p(z_1))-\lambda D_{KL}(\prod_{t=1}^{T}q_{\phi}(f_{g}|g)||\prod_{t=1}^{T}p(f_{g})\\\nonumber
%     &-\lambda D_{KL}(\prod_{t=1}^{T}q_{\phi}(f_{s}|s)||\prod_{t=1}^{T}p(f_{s})-\lambda D_{KL}(\prod_{t=1}^{T}q_{\phi}(f_{sg}|S_{1:T}, G_{1:T})||\prod_{t=1}^{T}p(f_{sg}) \\
% \end{align}

\subsection{Architectures \& Hyperparameters}
\label{sec:hyper}
Our model consists of four components which takes care of four types of latent variables $f_s$, $f_g$, $f_{sg}$, and $z_t$. To accommodate the disentangled information in each latent space and variance through time, we have four encoders, which models $q_{\phi}(f_s|S_{1:T},G_{1:T})$, $q_{\phi}(f_g|S_{1:T},G_{1:T})$, $q_{\phi}(f_{sg}|S_{1:T},G_{1:T})$, and $q_{\phi}(z_t|S_{1:T},G_{1:T})$, respectively. Each encoder learns a unique mean and standard deviation and each latent variable is randomly sampled from the Gaussian distribution, respectively. To encode the time-invariant spatial information via modelling $q_{\phi}(f_s|S_{1:T},G_{1:T})$, we implement a 1D convolution neural network. To encode the time-invariant graph information via modelling $q_{\phi}(f_g|S_{1:T},G_{1:T})$, we implement a typical graph convolution neural network \cite{kipf2016semi}. To encode the time-invariant spatial-graph correlated information via modelling $q_{\phi}(f_{sg}|S_{1:T},G_{1:T})$, we implement a spatial-graph convolution neural network~\cite{guo2021spatial}. To encode time-variant information, we implement another spatial-graph convolution neural network to capture the variance among different timesteps. With regard to decoders, we implement two decoders which one decodes the spatial information and the other one decodes the graph topological information. The input to the decoders are the concatenation of the latent presentation $f_s$, $f_g$, $f_{sg}$ and $z_t$. For example, to decode the graph topological information which includes nodes and edges, the input of the graph decoder is the concatenation of $f_g$, $f_{sg}$, and $z_t$. Similarly, to decode the spatial information, the input of the spatial decoder is the concatenation of $f_s$, $f_{sg}$, and $z_t$. To construct the edge feature or adjacency matrix, the input vector is mapped into a node-level feature vector through a fully connected layer first. Then, a matrix is constructed by replicating the vector. The edge's hidden representation matrix is constructed from the latent representation by a node-to-edge deconvolution layer \cite{guo2018deep} which decodes each node-level representation by making sense of the contributions from each node to its related edge's hidden representation. Finally, the edge feature or adjacency matrix is constructed by an edge-edge deconvolution layer, which each hideden edge feature contributes to the generation of its adjacent edges. The spatial decoder is typical a set of 1D convolution layers. Similarly, the node features of the graphs are also generated by a set of typical 1D convolution layers. The detailed hyperparameters for encoders and decoders of our models are shown in Table \ref{tab:details_encoder} and Table \ref{tab:details_decoder}, respectively.

\subsection{Model Complexity Analysis}
\label{sec:time_analysis}
The proposed STND-VAE requires $O(N^2)$ time complexity for spatial-graph convolution, $O(N)$ time complexity for spatial convolution and $O(N)$ time complexity for typical graph convolution with respect to number of $N$ nodes in the graphs. In terms of encoders for time-variant features, our model amounts to $O(N^2)$ time complexity. In total, our model takes $O(N^2)$ time complexity, which is scalable compared to most of the existing graph generation models. For example, graphVAE \cite{simonovsky2018graphvae} amounts $O(N^4)$ time consumption in the worst case and graphRNN amounts $O(N^2)$ time complexity.

\begin{table*}
\caption{Encoders architectures (Each layers is expressed in the format of \textit{<filter\_size><layer type><Num\_channel><Activation function><stride  size>}. \textit{FC} refers to the fully connected layers). \textit{c-deconv} and  \textit{c-conv} refers to the cross edge deconvolution and convolution respectively. The activation functions after each layer are all ReLU except the last layers.}
    \centering
    \small
    \setlength\tabcolsep{2pt}
    \begin{tabular}{|l|l|l|l|l|l|l|}\hline
    \toprule
        Spatial Encoder& Joint Encoder&Graph Encoder&Time Encoder \\\hline
        Input: $L \in \mathbb{R}^{25\times 2}$ &Input: $E$, $L$ &Input: $E \in \mathbb{R}^{25\times25}$,$F\in \mathbb{R}^{25}$&Input: $E$, $L$ \\\hline
        $5$ conv1D.10. stride 1&S-MPNN.20& GCN.10&S-MPNN.20 \\\hline
        $5$ conv1D.10. stride 1&S-MPNN.50 &GCN.20&S-MPNN.50\\\hline
        $5$ conv1D.20. stride 1&FC.200.&FC.100.&FC.200.\\\hline
        FC.100.& FC.200&FC.100& FC.200\\\hline
        FC.100 & & &\\\hline        
    \end{tabular}
    \label{tab:details_encoder}
\end{table*}

\begin{table*}
\caption{Decoders architectures (Each layers is expressed in the format as \textit{<filter\_size><layer type><Num\_channel><Activation function><stride  size>}. \textit{FC} refers to the fully connected layers). \textit{c-deconv} and  \textit{c-conv} refers to the cross edge deconvolution and convolution respectively. The activation functions after each layer are all ReLU except the last layers.}
    \centering
    \small
    \setlength\tabcolsep{2pt}
    \begin{tabular}{|l|l|l|}\hline
    \toprule
        Graph Decoder(for edge)&Graph Decoder(for node) &Spatial Decoder \\\hline
        Input:$f_g\in \mathbb{R}^{100}$,$f_{sg}\in \mathbb{R}^{200}$,$z_{t}\in \mathbb{R}^{200}$  & Input:$f_g\in \mathbb{R}^{100}$,$f_{sg}\in \mathbb{R}^{200}$,$z_{t}\in \mathbb{R}^{200}$ &Input:$f_s\in \mathbb{R}^{100}$,$f_{sg}\in \mathbb{R}^{200}$,$z_{t}\in \mathbb{R}^{200}$\\\hline
        FC.500& FC.500 &FC.500 \\\hline
        $5$ conv1D.50. stride 1 &$5$ conv1D.50. stride 1&$5$ conv1D.50. stride 1\\\hline
        $5\times5$ deconv.20. stride 1&$5$ conv1D.20. stride 1 &$5$ conv1D.20. stride 1\\\hline
        FC.1 &FC.1&$5$ conv1D.10. stride 1\\\hline
        &&FC.2 \\\hline        
    \end{tabular}
    \label{tab:details_decoder}
\end{table*}

% \begin{table*}
% \caption{Regularization term weights.}
%     \centering
%     \small
%     \setlength\tabcolsep{2pt}
%     \begin{tabular}{|l|l|l|l|}\hline
%     \toprule
%         $\beta_1$ & $\beta_2$ & $\beta_3$ & $\beta_4$ \\\hline
%         1.0 & 1.0 & 1.0 & 1.0
%         \\\hline  
%     \end{tabular}
%     \label{tab:details_decoder}
% \end{table*}

\subsection{Dataset}
\label{sec:app_dataset}
\textbf{Dynamic Waxman Random Graphs.}
The dynamic Waxman random graphs are generated by uniformly placing $n$ nodes at random in a rectangular domain \cite{waxman1988routing} through a time sequence $t$. First, the graph edge connection is modeled by pairwise distance $d$ between any two nodes with an edge probability of $\beta{e}^{-d/\alpha L}$, where $L$ is the maximum distance between any pair of nodes, and $\alpha$, $\beta$ are predefined parameters\footnote{The default parameters in Networkx \cite{hagberg2008exploring} package are $\beta$ as 0.4 and $\alpha$ as 0.1.}. Second, the spatial locations of the nodes are uniformly generated within the rectangular domain, where the coordinates of the four vertexes of the rectangular domain for generating the spatial locations of the nodes are $(p,p)$, $(p,p+n\times s)$, $(p+n\times s,p)$, $(p+n\times s,p+n\times s)$, respectively. Here the absolute position of the graphs is ranged from $1$ to $11$, and the location density of the nodes is ranged from $4$ to $11$. The node attribute, i.e. node color, is sampled from a random Gaussian distribution with mean $b$ ranging from $1$ to $11$. Finally, the temporal attributes are modeled by multiplying a time factor associated with a node attribute, i.e. node size. In the end, we have four types of latent factors corresponding to semantic factors in the dynamic Waxman random graphs dataset, which the graph-exclusive factor $b$ controlling node color semantic factor, the spatial-exclusive factor $p$ controlling the node spatial location semantic factor, the spatial-graph correlated factor $s$ controlling graph and spatial density, and the time-variant factor $t$ controlling node size varying through the sequence. In total, we have 2500 sequences of length 8 for training and 500 sequences of length 8 for testing.

\textbf{Dynamic Random Geometry Graphs.}
The dynamic random geometry graphs are generated by uniformly placing $n$ nodes at random in a rectangular domain \cite{bradonjic2007giant} through a time sequence $t$. First, the graph topology is modeled by pairwise distance $d$ larger than a threshold $\theta$ between any two nodes with an edge\footnote{$\theta$ parameter is set as 12 in our experiment}. Similarly, the spatial locations and temporal attributes are generated in the same way as in the dynamic Waxman random graphs. Finally, we have four types of latent factors corresponding to semantic factors in the dynamic random geometry graphs dataset, which the graph-exclusive factor $b$ controlling node color semantic factor, the spatial-exclusive factor $p$ controlling the node spatial location semantic factor, the spatial-graph correlated factor $s$ controlling graph and spatial density, and the time-variant factor $t$ controlling node size varying through the sequence. In total, we have 2500 sequences of length 8 for training and 1000 sequences of length 8 for testing.

\textbf{Protein Folding Dataset.}
Protein structures are naturally spatial graphs, which each node represents an amino acid with a spatial location and edge represents contacts between two amino acids ($d < 8$ \AA). The protein folding dataset includes a series of protein structures representing the folding process of a protein sequence $AGAAAAGA$ of length 8. In the protein folding dataset \cite{guo2020interpretable}, the graph density (reflected by the density of the inter-residue contacts) and the folding degrees (reflected by spatial locations of amino acids) of protein are spatial-graph correlated factors. The folding phrase ranging from 1 to 1000 represents temporal attributes during the folding process. In total, we have 4750 of length 8 for training and 4750 sequences of length 8 for testing.

\textbf{Traffic Dataset MERT-LA.}
Traffic data is one of the most common data type to study spatiotemporal graphs. MERT-LA \cite{jagadish2014big} is collected by Los Angeles Metropolitan Transportation Authority(LA-Metro), and processed by University of Southern California's Integrated Media Systems Center. This dataset contains traffic information collected from loop detectors in the highway of Los Angeles County by 207 sensors for four continuous months (from Mar 1-st 2012 to Jun 30-th 2012). We set one time step as one hour and total number of time steps in one sequence as 4. For the total of 714 samples, 500 samples are used for training and 214 samples are used for testing.

\subsection{Evaluation Metrics}
\textbf{avgMI}: Specifically, a mutual information matrix is constructed which measures the mutual information between the latent variables $f_s$, $f_g$, $f_{sg}$, $z_t$, and the expected spatial, graph, spatial-graph correlated semantic factors. Then the avgMI score calculates the mean squared error between the calculated mutual information matrix and the "gold-standard" mutual information matrix, which is a unit diagonal matrix.
